# Supplementary material for: Querying in Constant Expected Time with Learned Indexes
Source: arXiv:2405.03851 source file (2024-10-22)
Supplement: Supplementary file 1 [file appendix-F.tex]

\subsubsection{Lower bounds}
\label{sec:4-lower-bounds}

The results proved so far provide an upper bound for the complexity of searching with learned indexes. In particular, Theorem \ref{thm:constant-time} shows that expected query time can be achieved with \textit{at most} $O(n)$ space cost. To provide a more complete theoretical understanding of learned indexes, we now provide a lower bound on complexity. More specifically, we show that for a certain class of learned indexes, \textit{at least} $\Omega(\sqrt{n})$ space is needed to get expected query time.

Let $\T$ denote the class of learned indexes which can be represented as trees with the following characteristics. Structurally, each learned index is such that: (i) the corresponding tree is rooted; (ii) each non-leaf node stores a predictive model; and (iii) each leaf node stores an integer.
% ranging from $1$ to $n$ (where $n$ is the number of keys).
On the other hand, the search operation for any query parameter $q$ is such that: (i) it can be represented as a path starting at the root of the tree and ending in a leaf; (ii) at each non-leaf node, the predictive model plus a local search determines which child node is visited next in the path; and (iii) once a leaf is reached, the integer stored in the leaf corresponds to $\rank(q)$ and is returned.

Note that many, if not most, 1-dimensional learned indexes fit within the above description \cite{kraska2018case, ferragina2020pgm, ding2020alex, galakatos2019fiting, zeighami2023distribution}, including the ESPC index. For all learned indexes in $\T$, we can derive a lower bound on the space requirements needed to achieve constant expected query time.

\begin{theorem}
    Let the stochastic process $X = \{X_i\}_{i \in \mathbb{N}}$ be such that the $X_i$ are jointly independent random variables. Moreover, let all $X_i$ and the query parameter $q$ be characterized by a density $f$ with support $[a, b]$ and $\rhohf < \infty$. Let $R_n$ be a procedure for building learned indexes such that its codomain is $\T$. Then, $\timen=O(1)$ implies that $\spacen \geq 2^{h_1(X_1)}\sqrt{(b-a)n} = \Omega(\sqrt{n})$, where $h_1$ denotes the differential entropy.
\end{theorem}

\begin{proof}
    Our proof makes use of rate-distortion theory \cite{shannon1959coding, davisson1972rate}, the area within information theory which studies the theoretical properties of lossy data compression. The key observation is that a learned index can be used to derive an approximate representation of the random variable $q$. Then, rate-distortion theory can be used to relate the quality of this approximation to certain properties of the learned index.
    
    Let $A=[\osx{1}, \ldots,\osx{n}]$ be the sorted array formed by the first $n$ variables in the stochastic process $X$. Let $\tree = R_n(A)$ be the learned index which can be used to compute $\rank(q)$. Since the codomain of $R_n$ is $\T$, we know that $\tree\in\T$. We now introduce some notation regarding this structure.
    
    Since $\tree\in\T$, we know $\tree$ is rooted and for each node $v$ we can define its \textit{level} $\level(v)$ as the length of the path going from the root to $v$. The \textit{height} of the tree is correspondingly defined as $h(\tree) = \max_{v\in\tree} \level(v)$, where $v\in\tree$ is used to denote that $v$ is a node in $\tree$. Furthermore, we define $\C(v)$ as the set of children of node $v$. We call $|C(v)|$ the \textit{branching factor} at node $v$ and use $B(\ell)$ to denote the maximum branching factor at level $\ell$, that is:
    \begin{equation*}
        B(\ell) = \max \{|C(v)| \text{ such that } v\in\tree, \level(v)=\ell\}.
    \end{equation*}

    Now, consider a query parameter $q$ distributed according to the same density $f$ as the $\{X_i\}$. Since $\tree\in\T$, we know we can use $\tree$ to compute $\rank_{A}(q)$ and we know that the computation involves a traversal starting at the root of the tree and ending at some leaf. Denote by $v_0, \ldots, v_d$ the nodes visited during this traversal, such that $v_0$ is the root, $v_d$ is the leaf, and each $v_\ell$ is at level $\ell$.
    
    The exact path $v_0, \ldots, v_d$ traversed during the computation of $\rank_A(q)$ will depend on the exact value of the random variable $q$. Nonetheless, we can represent it as a tuple $P(q)$ defined as
    \begin{equation*}
    P(q)
    =
    \Big(
        (c_0, \eps_0, b_0),
        \ldots,
        (c_{d-1}, \eps_{d-1}, b_{d-1})
    \Big).
    \end{equation*}
    For each level $\ell$, the value $c_\ell$ represents which child would be visited according to the predictive model, $\eps_\ell$ denotes the magnitude of the correction determined by the local search (i.e., the corrective step), and $b_\ell$ is a single bit which describes whether the correction term $\eps_\ell$ should be added or subtracted from $c_\ell$.
    
    Now, we can define the following procedure to approximately represent $q$.

    \pagebreak

    We first provide a high-level and intuitive description of our argument. We know that for any query parameter $q$, the index can be used to determine $\rank(q)$, which can take any integer value in $\{0,\ldots,n\}$. In other words, the output of the index needs to specify at least $\log_2 n$ bits of information. Now, looking at it in a different way, notice that the output of the index can be fully specified by:
    \begin{enumerate}
        \item Indicating the leaf $k\in\{1,\ldots,K\}$ of the index tree structure corresponding to the search operation with input $q$. This requires $\log_2 K$ bits.
        \item Indicating which position within the $k$-th subarray corresponds to $\rank(q)$. Not all subarrays are the same size, so as a general matter, the position within any subarray can be fully specified with $\log_2 \left(\max_K \Delta_K\right)$ bits.
    \end{enumerate}
     Putting both lines of reasoning together, the following inequality must hold:
    \begin{equation}
    \label{eq:rate-distortion-inequality-informal}
        \log_2 K + \log_2 \left(\max_K \Delta_K\right) \geq \log_2 n
        \implies
        K \geq \frac{n}{\max_K \Delta_K}.
    \end{equation}
    Now, we can use this last expression to derive lower bounds for the space used by the index, in the following way. Suppose we are interested in achieving $O(1)$ expected query time. As the sizes of the subarrays grow larger, it is reasonable to suppose that the approximation error and by extension, the query time, go up. So we can aim to show that $O(1)$ expected query time requires $\max_K \Delta_K = O(a(n))$ for some function $a$. By (\ref{eq:rate-distortion-inequality-informal}) this implies
    \begin{equation}
        K = \Omega\left(\frac{n}{a(n)}\right).
    \end{equation}
    For instance, $a(n)=\sqrt{n}$ means $K=\Omega(\sqrt{n}))$, proving that at least square root space is needed to achieve $O(1)$ expected time.

    The central part of our argument revolves around the fact that an index as defined constitutes an approximate representation 

    Notice that an index as defined can be used to build an approximate representation of a query parameter $q$. Indeed, consider the following procedure:
    \begin{enumerate}
        \item Use the learned index to find $i = \rank(q)$.
        \item Return $\hat{q} = A[i] = \osx{i}$.
    \end{enumerate}
\end{proof}

\newpage

\begin{figure}[ht]
    \centering
    \includegraphics[width=1\linewidth]{
        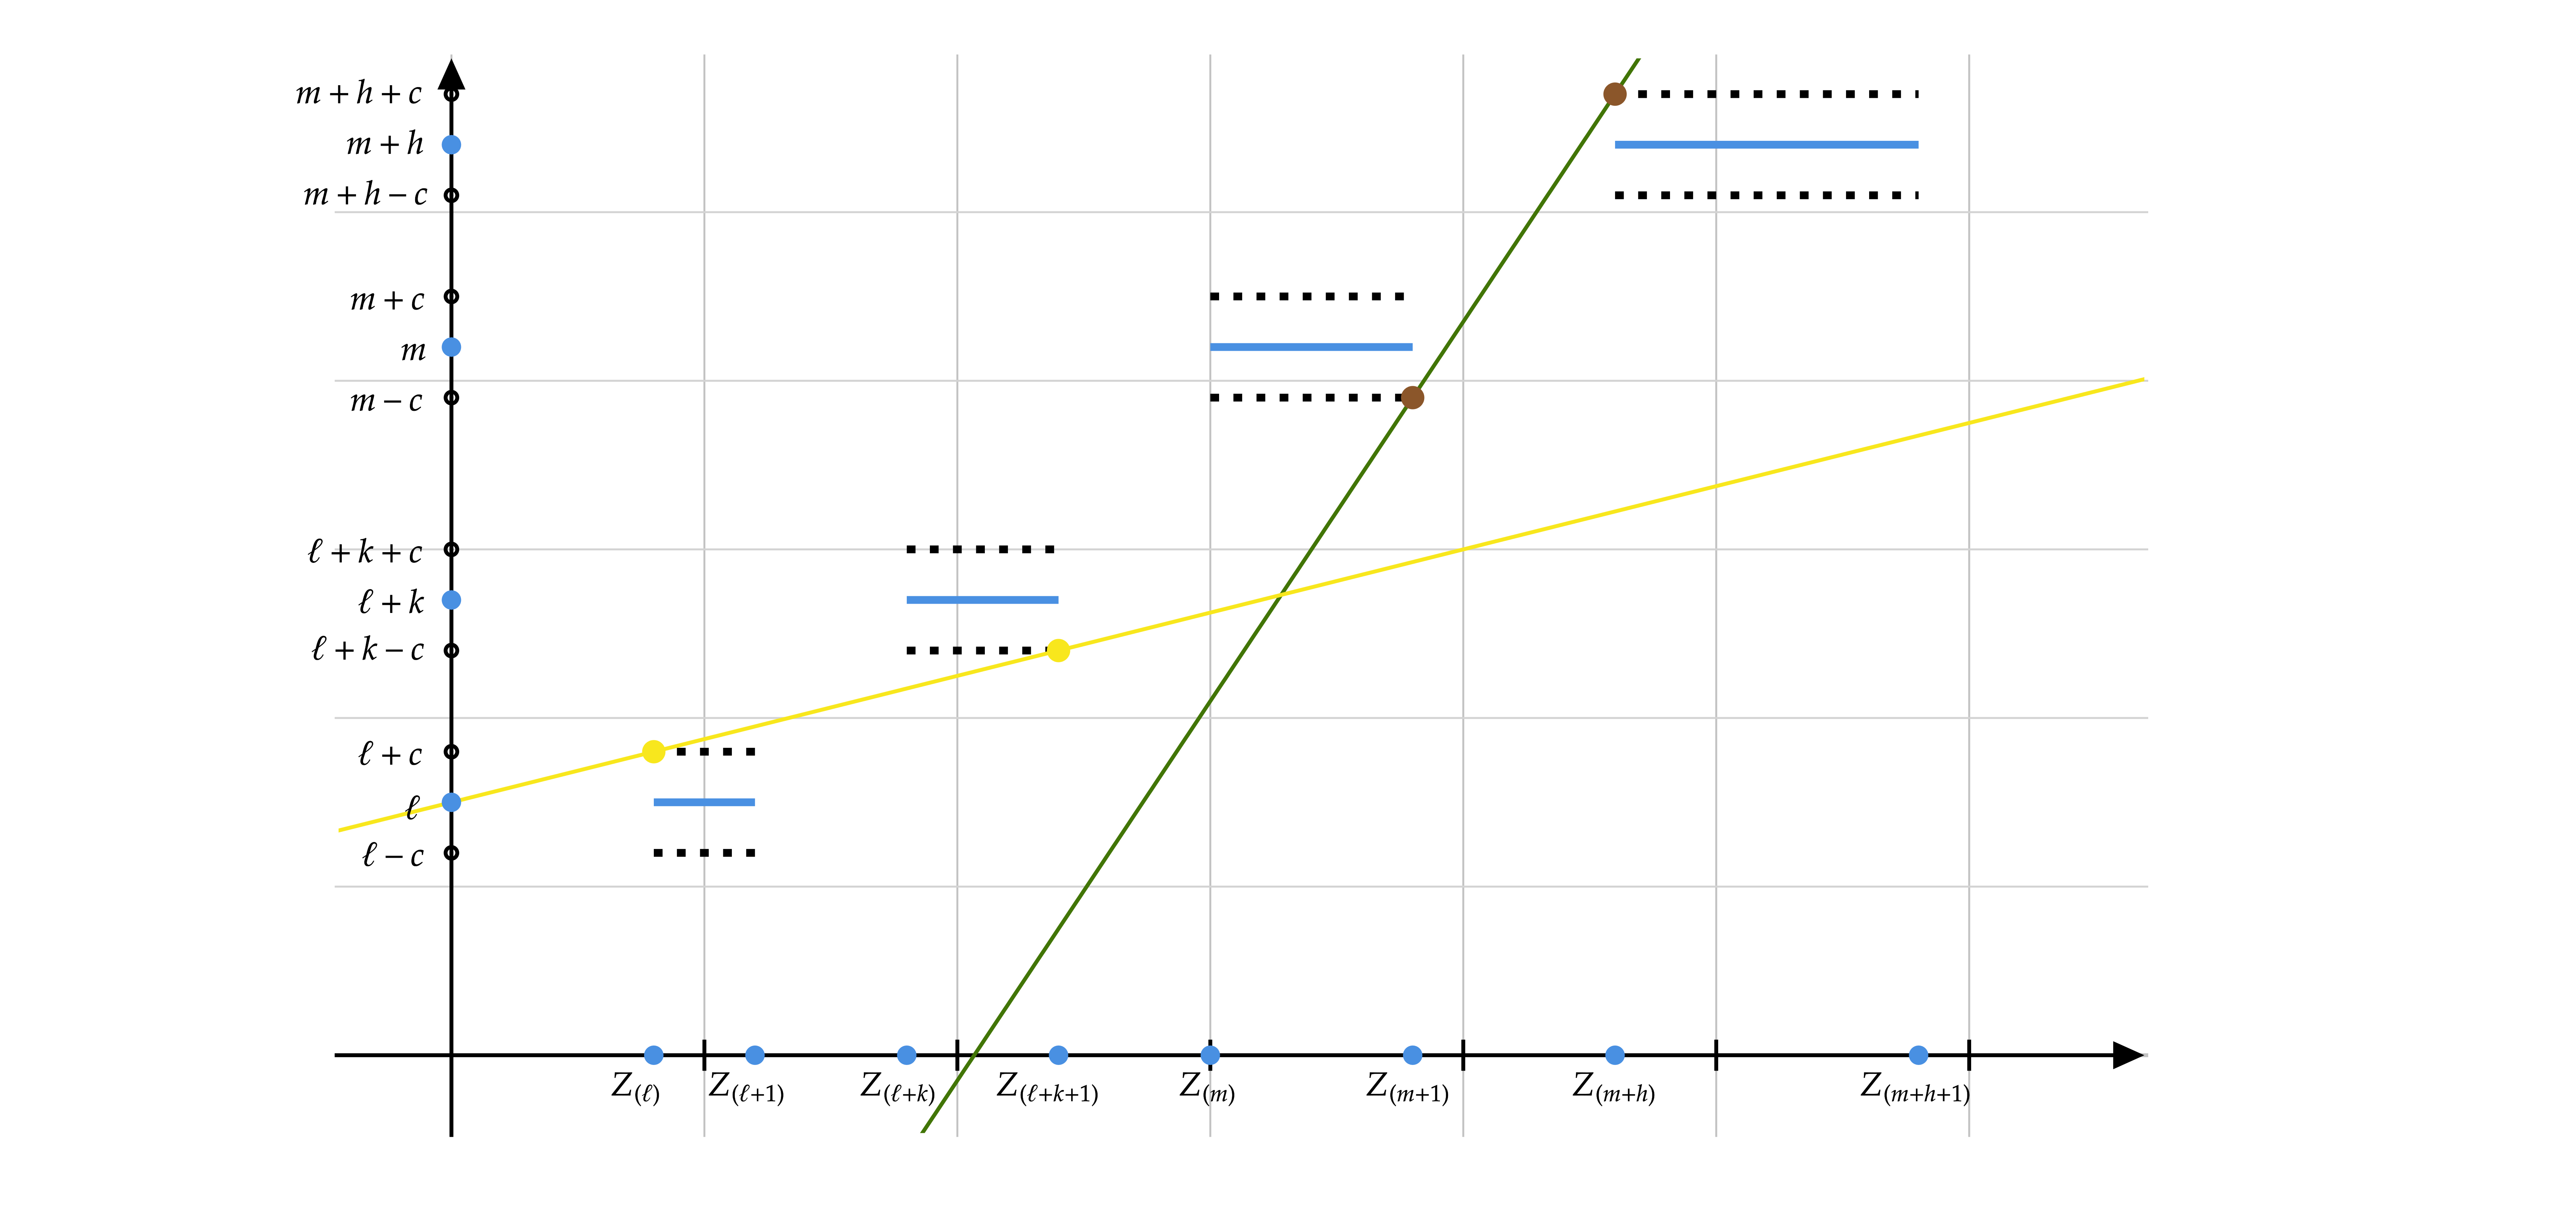
    }
    \caption{}
    \label{fig:order-statistics-and-slope}
\end{figure}

Consider an interval $I_k$ spanning the keys $\{\osx{i_k},\osx{i_k+1},\ldots,\osx{j_k}\}$. For the type of index we are considering, each interval has a linear model that approximates the rank function within that interval. In other words, there is a linear model $L_k(q) = a_k q + b_k$ that is used to approximate $\rank(q)$ for $q\in [\osx{i_k}, \osx{j_k}]$. We are interested in the quality of this approximation. Specifically, consider the metric
\begin{equation*}
    \Delta_i
    = \min_{q\in [\osx{i}, \osx{i+1}]} |L_k(q) - i|
\end{equation*}
defined for all $i\in \{i_k, \ldots, j_k-1\}$. Notice that the minimum is well-defined since $|L_k(q) - i|$ is a continuous function and $[\osx{i}, \osx{i+1}]$ is a compact set. Since $\rank(q)=i$ for $q\in [\osx{i}, \osx{i+1})$, the metric $\Delta_i$ quantifies the minimum error for the linear approximation of $\rank$ within this interval. In particular, suppose $\Delta_i > c$ for some $c>0$. Then, it holds that
\begin{align*}
    \expec{\eps \>|\> q\in [\osx{i}, \osx{i+1}]}
    &= \int_{\osx{i}}^{\osx{i+1}} |L_k(q) - \rank(q)| \densityx(q) dq \\
    &= \int_{\osx{i}}^{\osx{i+1}} |L_k(q) - i| \densityx(q) dq \\
    &> c \int_{\osx{i}}^{\osx{i+1}} \densityx(q) dq \\
    &= c \int_{\osx{i}}^{\osx{i+1}} e^{-q} dq \\
    &> c \int_{\osx{i}}^{\osx{i+1}} (1-q) dq \\
    &= c \left(\osx{i+1}-\osx{i}\right) - \frac{c}{2}\left(\osx{i+1}^2-\osx{i}^2\right) \\
    &= c \left(\osx{i+1}-\osx{i}\right)\left(1-\frac{\osx{i}}{2}-\frac{\osx{i+1}}{2}\right)
\end{align*}

Now take any $c>0$ and let $J$ denote the lower half of the $\{i_k, \ldots, j_k\}$ set of indices. Now, consider the following two possible scenarios:
\begin{enumerate}
    \item First, suppose $\Delta_i > c$ for all $i\in J$. Then, it follows that
    \begin{equation*}
        \expec{\eps \>|\> q\in I_k}
        \geq c \sum_{i\in J}\int_{\osx{i}}^{\osx{i+1}} \densityx(q) dq.
    \end{equation*}
    \item Otherwise, suppose there exists $\ell\in J$ such that $\Delta_\ell\leq c$. Then, we can lower bound $\expec{\eps \>|\> q\in I_k}$ in the following way.
\end{enumerate}

Consider the schematic in Figure \ref{fig:order-statistics-and-slope}. Given that $\Delta_\ell\leq c$, we are interested in the event $\Delta_{m+h}\leq c$. We can show that for $c=\log n$, with $m, \ell \geq \frac{n}{2}$ such that $m-\ell\geq \sqrt{n\log n}$, and taking $k=h=\sqrt{n\log n}$, we get
\begin{equation*}
    \prob{\Delta_{m+h}\leq c} \leq \frac{1}{2}
    \implies \prob{\Delta_{m+h}> c} \geq \frac{1}{2}.
\end{equation*}

So, we can take 

\begin{align*}
    \expec{\eps}
    &= \sum_{i=1}^n \expec{\eps | q\in I_i}\prob{q\in I_i} \\
    &= \sum_{i=1}^n \prob{q\in I_i} \int_{0}^\infty \eps(q) f_{X | X\in I_i}(q)dq \\
    &= \sum_{i=1}^n \prob{q\in I_i} \int_{0}^\infty \eps(q) \frac{d}{dq}F_{X | X\in I_i}(q)dq \\
    &= \sum_{i=1}^n \prob{q\in I_i} \int_{0}^\infty \eps(q) \frac{d}{dq}\prob{t\leq q | t\in I_i}dq \\
    &= \sum_{i=1}^n \int_{0}^\infty \eps(q) \frac{d}{dq}\prob{t\leq q \cap t\in I_i}dq
\intertext{If $q\leq \osx{i}$ then $\prob{t\leq q \cap t\in I_i}=0$ with corresponding $0$ derivative. If $q\geq \osx{i+1}$ then $\prob{t\leq q \cap t\in I_i}=\prob{t\leq q}$ with corresponding .}
\end{align*}

Otra forma

\begin{align*}
    \expec{\eps}
    &= \int_{0}^\infty \eps(q) f(q)dq \\
    &= \sum_{i=1}^n \int_{\osx{i}}^{\osx{i+1}} \eps(q) f(q)dq \\
    &\geq \sum_{i=1}^n c \mathbf{1}_{\Delta_i \geq c}\int_{\osx{i}}^{\osx{i+1}} e^{-q}dq \\
\intertext{With high probability:}
    &\geq \frac{c}{n}\sum_{i=1}^n \mathbf{1}_{\Delta_i \geq c}(\osx{i+1} - \osx{i})
\end{align*}
